# Supplementary material for: Collaborative Regression of Expressive Bodies using Moderation
Source: arXiv:2105.05301 source file (2021-10-15)
Supplement: Supplementary file 1 [file supmat_FIG_02_MoreQUAL.tex]

\begin{figure*}
 	\centering
    \includegraphics[width=1.00\textwidth]{figures/FINAL_PIXIE_vs_FrankMocap_no3_v2.png}

     \caption{
 				Qualitative \modelname results and comparison to \expose \cite{Choutas2020_expose} and \frankmocap \cite{rong2020frankmocap}.
 				From left to right:
 				(1) \rgb image,
 				(2) \expose \cite{Choutas2020_expose},
 				(3) \frankmocap \cite{rong2020frankmocap},
 				(4) \modelname \threeD body predictions \tdv{with estimated albedo and lighting}. 
 			% 	(5) \modelname with estimated albedo and lighting.
 				Our model improves upon existing expressive body estimation methods, by estimating 
 				(i)	    more visually plausible body shapes, through implicit reasoning about gender, and 
 				(ii)	better facial expressions and details, by leveraging insights from the \threeD face community. 
 	}
 	\label{fig:qual_sup_mat}
 \end{figure*}
